# Supplementary material for: Introduction into Calculus over Banach algebra
Source: arXiv:1601.03259 source file (2017-09-12)
Supplement: Supplementary file 1 [file Appendix.16.Calculate.Russian.tex]

%auto-ignore

\input{Appendix.16.Calculate.Eq}

\Chapter{Вспомогательные расчёты}

Я поместил в этом приложении расчёты,
которые необходимы для формирования некоторых утверждений.
Но я не хотел, чтобы эти расчёты заслоняли основную логику текста.

\Section{Расчёты для оценки интеграла (\ref{eq: int h2=int 12 xx+})}

Упростим подынтегральное выражение интеграла
\EqRef{int h2=int 12 xx+}
\ShowEq{int h2=int 12 xx+ 1}
Равенство
\ShowEq{int h2=int 12 xx+ 2}
является следствием равенства
\EqRef{int h2=int 12 xx+ 1}.
Равенство
\ShowEq{int h2=int 12 xx+ 21}
является следствием равенства
\EqRef{int h2=int 12 xx+ 2}.
Равенство
\ShowEq{int h2=int 12 xx+ 3}
является следствием равенства
\EqRef{int h2=int 12 xx+ 21}.
Равенство
\ShowEq{int h2=int 12 xx+ 4}
является следствием равенства
\EqRef{int h2=int 12 xx+ 3}.
Равенство
\ShowEq{int h2=int 12 xx+ 5}
является следствием равенства
\EqRef{int h2=int 12 xx+ 4}.

\Section{Расчёты для оценки интеграла (\ref{eq: int h2=int 12 3x2})}

Упростим подынтегральное выражение интеграла
\EqRef{int h2=int 12 3x2}
\ShowEq{int h2=int 12 3x2 1}
Равенство
\ShowEq{int h2=int 12 3x2 2}
является следствием равенства
\EqRef{int h2=int 12 3x2 1}.
Равенство
\ShowEq{int h2=int 12 3x2 3}
является следствием равенства
\EqRef{int h2=int 12 3x2 2}.

\ePrints{1601.03259}
\ifx\Semafor\ValueOn
\Section{Пример дифференциальной формы}
\else
\Section{Дифференциальная форма в поле комплексных чисел}
\fi
\labelSection{differential form in complex field}

Согласно теореме
\RefTheorem{omega=aE+bI is integrable},
дифференциальная форма
\DrawEq{omega=aE+bI}{example}
интегрируема тогда и только тогда, когда
\DrawEq{d omega=0 condition}{example}
Положим
\ShowEq{a=x2}
Равенство
\ShowEq{da/d}
является следствием равенства
\EqRef{a=x2}.
Равенство
\ShowEq{da dx0+dx1}
является следствием равенства
\EqRef{da/d}.
Равенство
\ShowEq{db -dx0+dx1}
является следствием равенств
\eqRef{d omega=0 condition}{example},
\EqRef{da dx0+dx1}.
Положим
\ShowEq{db/dx0=0}
Уравнение
\ShowEq{db/dx1=}
является следствием равенств
\EqRef{db -dx0+dx1},
\EqRef{db/dx0=0}.
Равенство
\ShowEq{b=x1x1}
является следствием уравнения
\EqRef{db/dx1=}.
Равенство
\ShowEq{omega(x)= example}
является следствием равенств
\eqRef{omega=aE+bI}{example},
\EqRef{a=x2},
\EqRef{b=x1x1}.

Пусть отображение
\ShowEq{f:A->B}fCC
является интегралом дифференциальной формы
\EqRef{omega(x)= example}
\ShowEq{f=int o}
Уравнения
\ShowEq{df dx0 dx1}
являются следствием равенств
\EqRef{df/dx= complex field},
\EqRef{omega(x)= example}.
Уравнения
\ShowEq{df a b}
являются следствием уравнений
\EqRef{df dx0 dx1 a},
\EqRef{df dx0 dx1 b}.
Равенство
\ShowEq{f(x0)+C(x1)}
является следствием уравнения
\EqRef{df dx0 a b}.
Уравнение
\ShowEq{dC/dx1}
является следствием равенств
\EqRef{df dx1 a b},
\EqRef{f(x0)+C(x1)}.
Равенство
\ShowEq{C(x1)=}
является следствием уравнения
\EqRef{dC/dx1}.
Равенство
\ShowEq{f(x)=}
являются следствием равенств
\EqRef{f(x0)+C(x1)},
\EqRef{C(x1)=}.
